# Supplementary material for: Room temperature p-induced surface ferromagnetism
Source: arXiv:1105.2777 source file (2011-05-13)
Supplement: Supplementary file 1 [file suppmat.pdf]

# Room temperature $p$-induced surface ferromagnetism – Supplementary Material

The *first-principles* calculations are performed within the density functional theory using two different approaches, the LSDA+U, as implemented in the pseudopotential SIESTA package [1], and the self-consistent Korringa-Kohn-Rostoker (KKR) method [2], involving local self-interaction corrections (LSIC) to treat localized electron states.

## SIESTA Calculations

In the SIESTA calculations the basis sets are constituted by multiple-zeta polarized localized numerical atomic orbitals (AO); for Zn we employ double-zeta (DZ) $s$ and $d$ AOs plus a single-zeta (SZ) $p$ AO, whereas for Oxygen DZ $s$ and $p$ AOs plus a SZ $d$ AO. The empirical Coulomb $U = 5.7$ eV and exchange $J = 1$ eV parameters were chosen to model the orbital dependent Hubbard-like potential for the Zn $d$ states [3]. We model the surfaces by a slab geometry, with slabs containing between 15 and 17 atomic planes along the crystallographic wurtzite $c$-axis and separated by a vacuum region of at least 20 Å were repeated periodically. Reciprocal space integration was performed on a $12\times12\times1$ Monkhorst-Pack supercell. Careful convergence in the $k$-mesh and the inclusion of relaxations are essential in order to accurately describe magnetism.

Dipolar corrections were applied for asymmetric slabs. Bulk-like behavior was always attained at the innermost central plane and the structure and electronic properties of the surfaces, both (0001) and $(000\bar{1})$, turned out to be independent of the symmetry of the slab. More details about the conditions of the calculations are found in Refs. [4, 5, 6].

The calculated in-plane $a = 3.25$ Å and out-of-plane $c = 5.20$ Å lattice parameters of ZnO are in good agreement with the experimental values [7] and we get a band gap of 1.25 eV. The O-ZnO $(000\bar{1})$ surface presents a compression of the O-Zn bond of $\approx 4\%$ and a smaller relaxation of the next two layer. Contrary, at the (0001) surface the O-Zn bond length is 2.04 Å which is slightly larger than the 1.98 Å of bulk bonds, although the large variations occur for the underneath bonds due to the outward relaxation of Zn atoms. The Zn-O pair distances, which present opposite relaxation, are 2.11 Å and 1.93 Å in the second and third layers, respectively. Subsequent layers retain their bulk structure.

The local DOS of the three topmost atoms, O$^1$, Zn$^1$, and O$^2$, are shown in Figure 1. There, one can see the large concentration of holes in the $p_z$

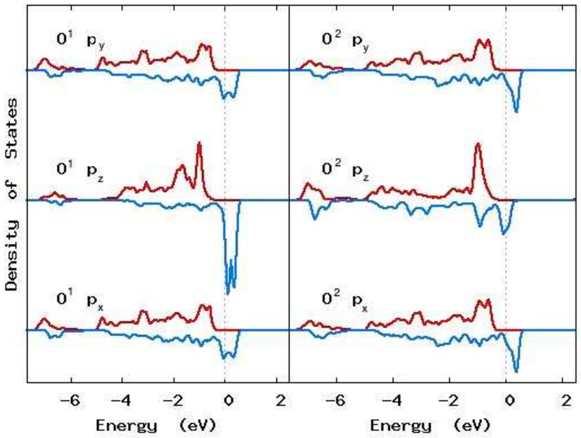


Figure 1: (Color online) Partial DOS of O$^1$ and O$^2$ from SIESTA calculations.

orbital of O$^1$ and the degeneracy of the $p_x$ and $p_y$ orbitals of both O atoms, as can be expected from symmetry.

The stability of the oxide surfaces depends on the partial oxygen pressure and hence it requires the calculation of the surface free energy as a function of the oxygen chemical potential. For a surface in thermal equilibrium with the oxygen gas, the surface free energy can be obtained from the *ab-initio* total energy combined with a thermodynamic formalism [8]. Figure 2 shows the relative surface free energies of the O-ZnO (0001) surfaces with the respective topmost oxygen at inequivalent positions, in the three-fold fcc hollow site (Oh) and on top of the Zn subsurface atom (Ot), as a function of the oxygen chemical potential. For negative/positive values the oxygen/zinc terminations are more stable. For comparison the relative surface free energy corresponding to the cleaved O-ZnO ($000\bar{1}$) surface is also represented. The figure indicates that for the complete allowed range of oxygen chemical potential the (0001) surface with O in the three-fold fcc hollow site is always more stable than the bulk-like termination Ot. Furthermore, for oxygen rich atmospheres the (0001) surface with O in the three-fold *fcc* hollow site is even more stable than the natural Zn-ZnO(0001) termination.

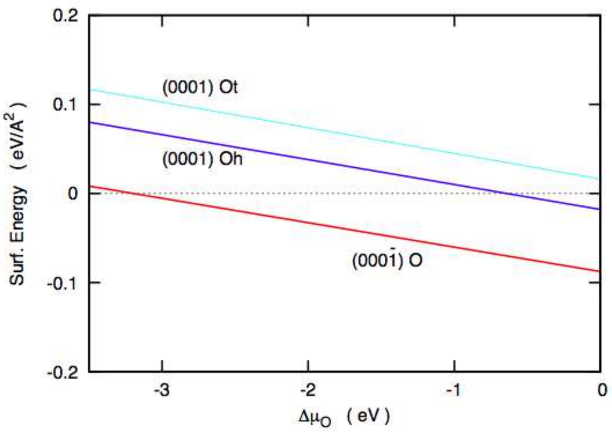


Figure 2: (color online) Relative surface free energies as a function of the oxygen chemical potential for the O-ZnO (000$\bar{1}$) (red line) and (0001) (blue lines) surfaces, with both, oxygen in the three-fold *fcc* hollow site (Oh) and at the bulk position on top of the Zn atom underneath (Ot).

## LSIC-KKR Calculations

For a more adequate description of the correlated electrons in the system, namely beyond that of local and semi-local approximations to DFT, the so-called local self-interaction correction (LSIC) approach, implemented within the framework of the multiple scattering Korringa-Kohn-Rostoker (KKR) method [2], has been employed to the relaxed (equilibrium) structures determined by SIESTA.

As in the LSIC-KKR method one deals with energy dependent quantities, a complex energy contour of 24 Gaussian quadrature points has been used in the calculations throughout, and for the Brillouin zone (BZ) integrations a 12x12x2 k-points mesh has been constructed. The crystal potential was constructed in the atomic sphere approximation. So-called empty spheres (ES) were used to improve space filling.

In doing so SIC was applied to all Zn $3d$ states, as this was shown to be the groundstate [9] in bulk ZnO. The resulting DOS of the LSIC-KKR calculation can be seen in Figure 3. It shows good agreement with the LSDA+U SIESTA calculations, shown in the main article. The main difference between the two approaches is that SIC pushes down the $3d$ electron states to much lower energies than LSDA+U does. The reason being that the self-

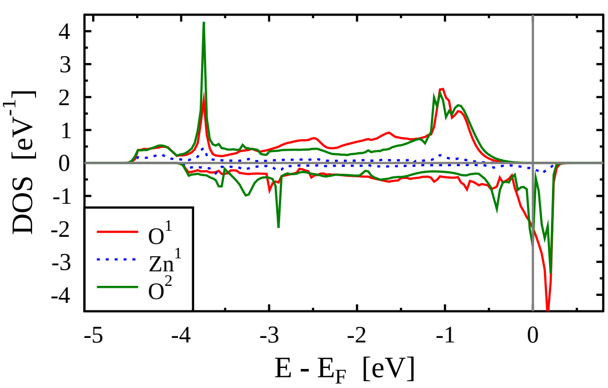


Figure 3: (color online) Local DOS of the 3 topmost atoms at the (0001)-h surface, resulting from KKR calculations with SIC on the $3d$ electrons of Zn.

interaction correction is applied only to the occupied states, which in terms of $U$ would amount to the shift in energy by its full unscreened value, while in the LSDA+U, by construction, the occupied states are shifted down only by $U/2$, with $U$ in most applications treated as an adjustable parameter. Note, here, that SIC has no adjustable parameters, but to make contact with spectroscopies the Slater transition state concept has to be implemented [10].

With respect to magnetic moment formation the results are well comparable, too, as can be seen in Table 1 in the middle row. There are only small differences. One can see that, compared to the SIESTA result, the relative strength of the MM of $O^1$ is smaller in the case of applying SIC to the Zn $3d$ states only. The sum of the shown values is slightly smaller. This is due to the usage of empty spheres, carrying weak magnetic moments, which make up for the difference.

Table 1: Magnetic moments (in $\mu_B$) for the topmost layers of the (0001) surface. The layers are labeled according to Fig. 1 in the paper.

| Method | $O^1$ | $Zn^1$ | $O^2$ |
|---|---|---|---|
| SIESTA | 0.94 | 0.01 | 0.53 |
| KKR (SIC on Zn $3d$ only) | 0.75 | 0.00 | 0.55 |
| KKR (SIC groundstate as in paper) | 1.06 | -0.06 | 0.42 |

For a more adequate description of the oxygen $p$ bands containing holes [11, 12, 13] LSIC has been applied to different symmetries and numbers of localized $p$ electron states on all the relevant oxygen atoms, in addition to all the Zn $3d$ electron states [9]. The global energy minimum, namely the LSIC groundstate, has been determined based on energetics, by inspecting a delicate energy balance between gain in band formation vs. localization. We have found that treating any majority $p$ spin orbital of $O^1$ as localized, by applying SIC, is energetically favourable. Applying SIC to all three majority $p$ electron states of $O^1$ is even more energetically favourable, making the total energy more negative, by $\approx 0.92\,\text{eV}$, with respect to the scenario where no SIC is applied to $p$'s of $O^1$ or any other oxygen atom. When SI- correcting more than three majority $p$ states on $O^1$, or any number of $p$ states on any other oxygen atom in the system, results in an energy loss, namely making the total energy more positive with respect to the scenario where only the Zn $3d$ states are treated as localized and thus self-interaction corrected. Consequently, the groundstate corresponds to the situation where all the Zn $3d$ states and all the majority $p$ electron states of $O^1$ benefit from localization and are SI-corrected.

The resulting MMs are shown in Table 1 in the bottom row. An increased MM on $O^1$ due to the increased localization of the SI-corrected majority bands is observed, causing an increased negative magnetization in the vicinity of the surface.

As described in the main article, the LSIC-KKR determined groundstate electronic structure has been used to investigate the magnetic interactions of the studied surfaces by applying the MFT. For this, we used the same complex energy contour of 24 points, convergence of the $J_{ij}$ with respect to the number of k-points is achieved with a 12x12x2 k-points mesh per energy point for the first 18 of them, and a 30x30x5 k-mesh for the last six energy points, lying close to the Fermi energy.

### Monte Carlo Simulations

The MC simulations have been performed by constructing lattices of 3200 to 4608 sites representing the two magnetic oxygen atoms. Importance sampling has been done using the Metropolis algorithm. During the simulations the system has been relaxed into equilibrium at a temperature $T$ above $T_C$. Then $T$ has been gradually reduced. At each $T$ point the system has been assumed to have reached equlibrium after 20,000 MC steps, after which measuring the

observables and averaging over further 20,000 MC steps has been done. $T_C$ has been obtained by inspecting the graphs of the susceptibility $\chi$, the specific heat $C_V$, and the so-called Binder cumulant $U_4$. All three quantities have delivered the same values for $T_C$. Further details about the $J_{ij}$ calculations via the MFT and the MC simulations are given in Ref. [14].

# References


[1] José M Soler, Emilio Artacho, Julian D Gale, Alberto García, Javier Junquera, Pablo Ordejón, and Daniel Sánchez-Portal. The SIESTA method for ab initio order-N materials simulation. *Journal of Physics: Condensed Matter*, 14(11):2745, March 2002.

[2] M. Lüders, A. Ernst, M. Däne, Z. Szotek, A. Svane, D. Ködderitzsch, W. Hergert, B. L. Gyorffy, and W. M. Temmerman. Self-interaction correction in multiple scattering theory. *Phys. Rev. B*, 71(20):205109, 2005.

[3] M. Khalid, M. Ziese, A. Setzer, P. Esquinazi, M. Lorenz, H. Hochmuth, M. Grundmann, D. Spemann, T. Butz, G. Brauer, W. Anwand, G. Fischer, W. A. Adeagbo, W. Hergert, and A. Ernst. Defect-induced magnetic order in pure ZnO films. *Phys. Rev. B*, 80(3):035331, Jul 2009.

[4] J. I. Beltrán, S. Gallego, J. Cerdá, J. S. Moya, and M. C. Muñoz. Bond formation at the Ni/$ZrO_2$ interface. *Phys. Rev. B*, 68(7):075401, Aug 2003.

[5] N. Sanchez, S. Gallego, and M. C. Muñoz. Magnetic states at the oxygen surfaces of ZnO and Co-doped ZnO. *Phys. Rev. Lett.*, 101(6):067206, Aug 2008.

[6] N. Sanchez, S. Gallego, J. Cerdá, and M. C. Muñoz. Tuning surface metallicity and ferromagnetism by hydrogen adsorption at the polar ZnO(0001) surface. *Phys. Rev. B*, 81(11):115301, Mar 2010.

[7] Ü Özgür, Ya. L. Alivov, C. Liu, A. Teke, M.A. Reshchikov, S. Dogan, V. Avrutin, S.-J. Cho, and H. Morko. A comprehensive review of ZnO materials and devices. *Journal of Applied Physisc*, 98(4):041301, August 2005.

[8] J. I. Beltrán, M. C. Muñoz, and J. Hafner. Structural, electronic and magnetic properties of the surfaces of tetragonal and cubic $HfO_2$. *New Journal of Physics*, 10(6):063031, 2008.

[9] I. V. Maznichenko, A. Ernst, M. Bouhassoune, J. Henk, M. Däne, M. Lüders, P. Bruno, W. Hergert, I. Mertig, Z. Szotek, and W. M. Temmerman. Structural phase transitions and fundamental band gaps of $Mg_x Zn_{1-x}O$ alloys from first principles. *Phys. Rev. B*, 80(14):144101, Oct 2009.

[10] Markus Däne, Martin Lüders, Arthur Ernst, Diemo Ködderitzsch, Walter Temmerman, Zdzislawa Szotek, and Wolfram Hergert. Self-interaction correction in multiple scattering theory: Application to transition metal oxides. *Journal of Physics: Condensed Matter*, 21:045604, 2009.

[11] Alex Zunger, Stephan Lany, and Hannes Raebiger. The quest for dilute ferromagnetism in semiconductors: Guides and misguides by theory. *Physics*, 3:53, Jun 2010.

[12] A. Droghetti, C. D. Pemmaraju, and S. Sanvito. Predicting $d^0$ magnetism: Self-interaction correction scheme. *Phys. Rev. B*, 78(14):140404, Oct 2008.

[13] W. A. Adeagbo, G. Fischer, A. Ernst, and W. Hergert. Magnetic effects of defect pair formation in ZnO. *Journal of Physics: Condensed Matter*, 22(43):436002, 2010.

[14] Guntram Fischer, Markus Däne, Arthur Ernst, Patrick Bruno, Martin Lüders, Zdzislawa Szotek, Walter Temmerman, and Wolfram Hergert. Exchange coupling in transition metal monoxides: Electronic structure calculations. *Phys. Rev. B*, 80(1):014408, 2009.
